# Supplementary material for: A Closer Look at the Explainability of Contrastive Language-Image Pre-training
Source: arXiv:2304.05653 source file (2024-09-16)
Supplement: Supplementary file 1 [file 6_suppl.tex]

\clearpage
%\setcounter{page}{1}
%\maketitlesupplementary
\appendix

\section{Extensive Examples of Opposite Visualization} \label{sup1}

\begin{figure}[h]
\centering
 \includegraphics{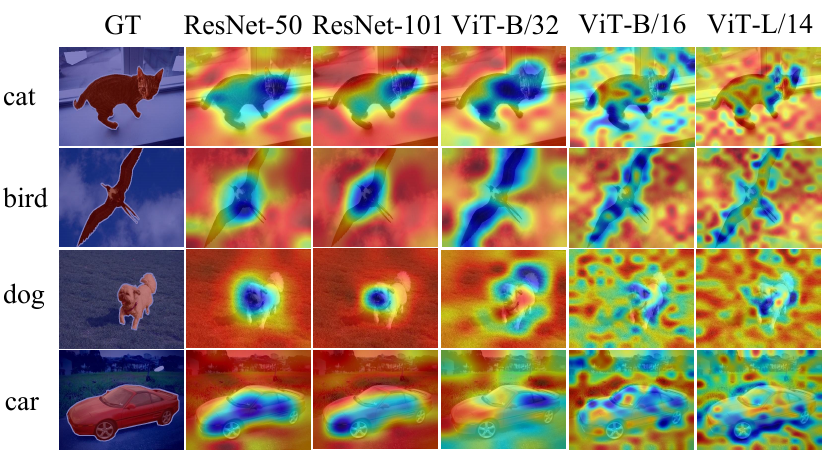}
\caption{CLIP shows opposite visualization against the ground truth ``GT" for both ResNets \cite{he2016deep} and ViTs \cite{dosovitskiy2020image}.}
\label{fig_prob1}
\end{figure}

We show more examples of opposite visualizations in Fig. \ref{fig_prob1}. This figure indicates the opposite visualization is universal to varied backbones. Besides, we noticed that the degree of opposite visualization would influence the significance of noisy activations as shown in Fig. \ref{pattern_change}.

\begin{figure}[h]
\flushright
 \includegraphics[width=8cm]{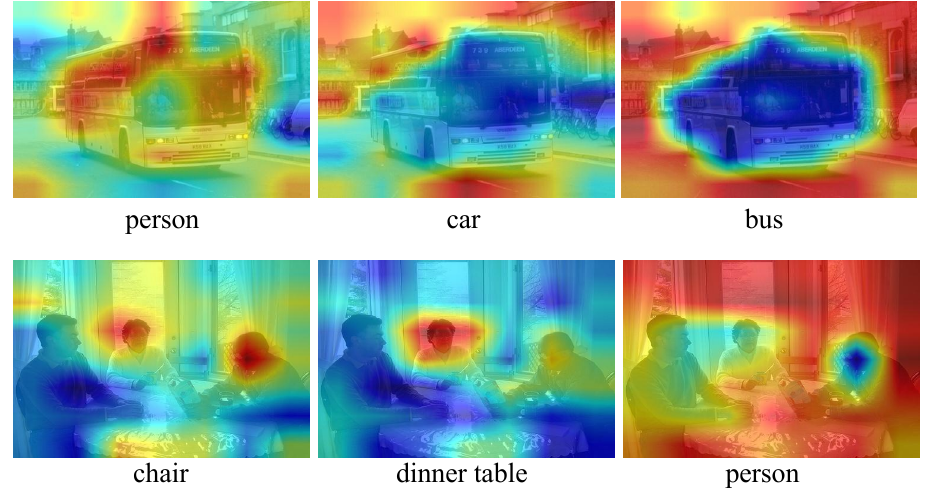}
\caption{ResNet-50 shows different noisy activation patterns (non-spot) when the opposite visualization is too serious.}
\label{pattern_change}
\end{figure}

\section{Quantitative Analysis of Opposite Self-attention Maps} \label{sup2}

Besides, visual analysis, we set quantitative analysis in Fig. \ref{fig_quantitive_attention}. Specifically, we quantitatively measure the ratio of attention on the foregrounds via the metric mean Foreground Self-attention Ratio (mFSR) as Eq. \ref{eq_mFSR}, where $m_c, m_s$ count the mean values along classes and samples (every positive labels on all images), respectively. Herein, $\boldsymbol{A} \in \mathbb{R}^{H \times W} (N_t = H \times W)$ is the self-attention averaged along the head dimension from the last layer (belonging to the token at the highest score on the similarity map), and $\boldsymbol{G}$ is the foreground binary ground-truth of each sample whose size is $H\times W$.

\begin{equation}
\label{eq_mFSR}
    mFSR = m_c(m_s(\frac{\sum_{i=1}^{H} \sum_{j=1}^{W} \boldsymbol{A}_{i,j} \cdot \boldsymbol{G}_{i,j}}{\sum_{i=1}^{H} \sum_{j=1}^{W} \boldsymbol{A}_{i,j}}))
\end{equation}

\begin{figure}[h]
\centering
\includegraphics[width=8.3cm]{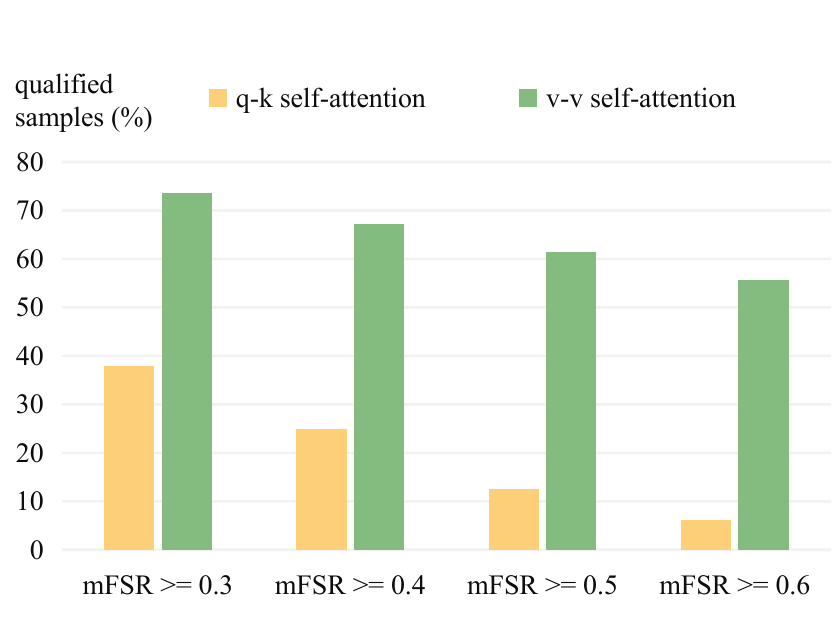}
\caption{Quantitative analysis towards the original q-k self-attention and the proposed v-v self-attention via the metric mean Foreground Self-attention Ratio (mFSR, higher value indicates more attention on the foregrounds). We show the qualified samples percentages (y-axis) at different mFSR ranges (x-axis) on VOC 2012 dataset \cite{everingham2010pascal} using backbone ViT-B/16. The results suggest our v-v self-attention mainly focuses on the foregrounds, but q-k self-attention prefers the backgrounds.}
\label{fig_quantitive_attention}
\end{figure}

Higher mFSR indicates the attention maps pay more attention on the foreground, while low mFSR indicates the self-attention link too much background towards the foreground tokens building an opposite relation. Notably, some information related to foreground are hard to involve into mFSR like attention around the boundary and related context. As a result, no specific mFSR value (e.g. 0.5) can indicate the foreground taking the lead. Thus, we set varied ranges of mFSR in Fig. \ref{fig_quantitive_attention}. If we regard the foregrounds taking the lead when mFSR is 0.3, 73.61\% samples are qualified in our v-v self-attention, while it's only 37.83\% for the original q-k self-attention. Especially for higher mFSR, the gaps are larger. Specifically, our results are 48.95\% and 49.39\% higher at mFSR 0.5 and 0.6, respectively. These results indicate the foreground tokens of the original CLIP take too much attention from the backgrounds  (e.g. 93.77\% samples prefer the background at mFSR 0.6), which leading to the opposite visualization.

This problem is also discussed in ECLIP \cite{li2022exploring}, their reason is the shifted feature in the pool layer. Different from it, we explore the underlying reason in the inference phase, instead of pooling layer in training. Here, we can correct erroneous self-attention for multiple layers in vision transformers \cite{dosovitskiy2020image} during inference, instead of the last pooling layer during training in ECLIP. Therefore, analyzing the self-attention helps us to correct explainability for multiple layers without training, and make it more readily applicable to downstream tasks without fine-tuning.

\section{Analyze for Multiple Modules} \label{sup3}

In this subsection, we aim to explain CLIP on the image-level predictions for multiple modules, besides pixel-level activations analyzed above. Foremost, we want to inform that all backbones of CLIP use the residual structure, where the last output is accumulated from multiple intermediate outputs. It means all intermediate outputs are directly contributed to the final decision thanks to the residual. Motivated by this principle, we aim to analyze each prediction summed in the residual and skip those outputs which are conflict to the final output for consistent explainability.

To interpret image-level predictions, we introduce the cosine of angle between text features and targeted image features, which is different from the analysis on self-attention. Specifically, we compute the cosine of angles $a<\ >$ between text feature $\boldsymbol{F}_i$ and image feature $\hat{\boldsymbol{F}_c}$ at the class token belonging to the targeted module (including self-attention modules and feed-forward networks (FFN) summed in the residual) as Eq. \ref{eq_cos_angle}. Note that each image feature is multiplied with the last linear projection layer to get $\hat{\boldsymbol{F}_c}$, and the class token is used to extract image-level features.
\begin{equation}
\label{eq_cos_angle}
    a<\boldsymbol{F}_t, \hat{\boldsymbol{F}_c}> = \frac{\boldsymbol{F}_t \cdot \hat{\boldsymbol{F}_c}}{\|\boldsymbol{F}_t\|_2 \cdot \|\hat{\boldsymbol{F}_c}\|_2}.
\end{equation}

\begin{figure}[h]
\centering
 \includegraphics[width=8.3cm]{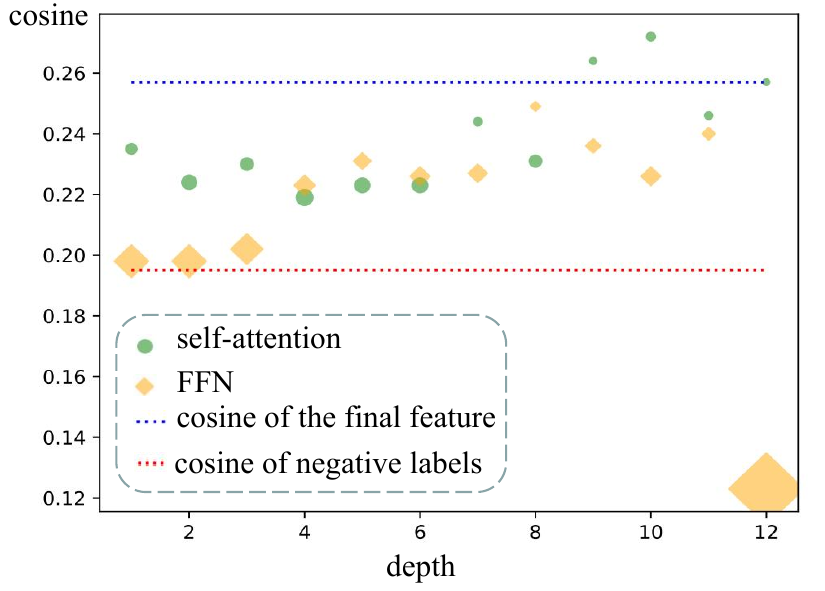}
\caption{Analysis for image-level intermediate predictions from self-attention blocks (green) and feed-forward networks (FFNs, colored in yellow) at different depths via the cosine of angles (Eq. \ref{eq_cos_angle}). The blue line indicates the mean cosine of all positive labels on VOC 2012 dataset \cite{everingham2010pascal} using backbone ViT-B/16, and the red line is that of negative labels. All scatters are the mean cosine of positive labels, and expected to be close to the blue line. Larger scatters indicate the features of this block are more inconsistent with the final prediction. Specifically, many FFN blocks are conflicted to the final predictions.}
\label{fig_cos_angle}
\end{figure}

Based on this metric, we set analysis for image-level intermediate predictions for multiple blocks involved in the residual at varied depth, then we draw the cosine of angles for each module in Fig. \ref{fig_cos_angle}. From this figure, we find FFN modules have larger gaps than self-attention modules, when computing the cosine of angle with the final classification feature. Especially, the last FFN returns the feature at cosine 0.1231, which is much farther than the cosine of negative labels. And features of first three FFNs are very close to the features of negative labels. This finding suggests that FFNs pushes features towards negatives when identifying positives, thus hurts the model. And Tab. \ref{tab_dual_paths} experimentally prove this claim in explainability task. Therefore, we only take features from the reformed self-attention modules without those of FFNs. Notable, this analysis is based on image-level features, which helps the design of architecture surgery for region-level explainability. Because the image classification uses the original path with the same classification performance, and the new path is not applicable to recognition task under fewer parameters.

\begin{figure}[h]
\centering
 \includegraphics[width=8.3cm]{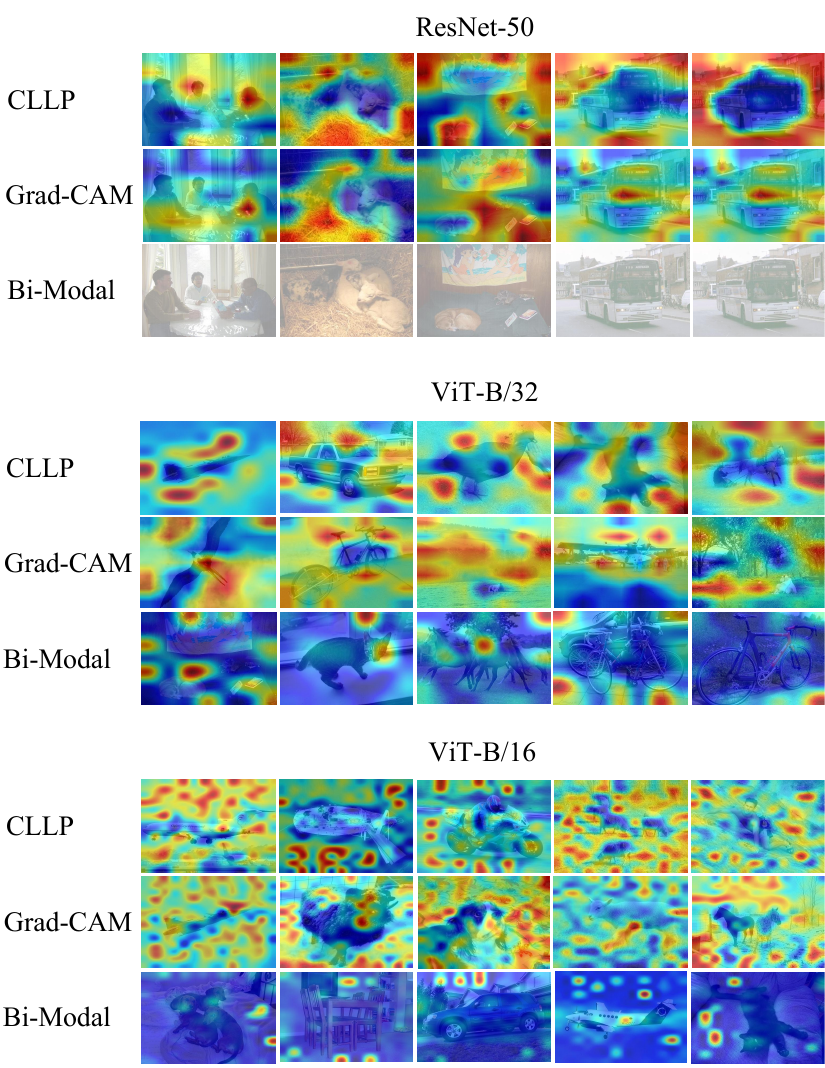}
\caption{Noisy activation is universal on the original CLIP for varied backbones and methods, including Grad-CAM \cite{selvaraju2017grad} for convolutional neuron networks and Bi-Modal \cite{chefer2021generic} for multi-modal vision transformers. These red activations on backgrounds are the noises at spot shape. The white mask indicates the explainability method designed for ViT is not applicable to ResNet. Note when the opposite visualization of ResNet is too obvious owing to unified features, the noisy activations are hard to observe.}
\label{fig_noisy_activations}
\end{figure}

\section{Noisy Activations are Universal in Different Backbones and Methods} \label{sup4}

As illustrated in Figure \ref{fig_noisy_activations}, this issue is conspicuous and raises concerns about the reliance of CLIP's decision-making on noisy regions instead of more discriminative areas. Furthermore, the noisy activations significantly degrade the quality of visualizations, resulting in spotty heatmaps with irregular shapes. It is therefore imperative that this issue is addressed in a careful and thorough manner. This issue is universal in different backbones and methods, which indicates it a common and important problem.

\section{Implementation Details} \label{sup5}
\label{sec_5.1.2}
For explainability task, we set experiments on the official CLIP with 5 backbones, namely ResNet-50, ResNet-101, ViT-B/32, ViT-B/16, ViT-L/14. For ResNets \cite{he2016deep}, CLIP adds an attention pooling with self-attention in the last layer, and their output size is 7 $\times$ 7 under input resolution 224 (all the datasets are resized to 224 $\times$ 224 without crop or other augmentation). For the output size of ViTs \cite{dosovitskiy2020image}, it depends on its patch size. Specifically, the output sizes are 7, 14, 16 for ViT-B/32, ViT-B/16, ViT-L/14, respectively. As for the hyperparameters of CLIP Surgery, the depth $d$ in Eq. \ref{eq_dual_paths} is set to 7, and softmax scale $\tau$ in Eq. \ref{eq_weight} is set to 2. Note, these hyperparameters are not sensitive with small variation of results. For example, on COCO 2017 \cite{lin2014microsoft} dataset using backbone ViT-B/16, the variation of results at metric mSC is 0.42\% for $d \in [1, 10]$, and variation for $\tau \in [1, 10]$ is 0.12\%. As to the textual prompt, we deploy the 85 templates in CLIP for ImageNet \cite{deng2009imagenet}, and combine templates with the names of categories. Then, we mean the text features along template dimension as the final text features $F_t$, and this prompt ensemble is applied to all methods for fair comparison. 

For open-vocabulary semantic segmentation, we resize the images of PASCAL Context \cite{mottaghi2014role} and COCO Stuff \cite{caesar2018coco} to 512 $\times$ 512, and crop each image of Cityscapes to 8 patches at 512 $\times$ 512 from 2048 $\times$ 1024 without overlap. For fair comparison, all the compared methods use the same backbone ViT-B/16, except grouping methods \cite{xu2022groupvit,luo2022segclip} whose backbones are specially designed. Note, the original ReCo \cite{shin2022reco} uses ResNet50x16 which is much larger than ViT-B/16, and the implemented results based on ViT-B/16 are from the official code. Since ViL-Seg \cite{liu2022open} is not released, we report its results from the paper. And we reproduce the results of MaskCLIP \cite{zhou2022extract} at the same settings as ours, without its post-processing methods, for fair comparison with other works. For open-vocabulary multi-label recognition, we take the prediction from the original path (the same as original CLIP at input size 224), and apply feature surgery to replace the softmax operation of CLIP. For other CLIP-based zero-shot methods \cite{sun2022dualcoop,xu2022dual,he2022open}, we report their results from the papers. Besides, we implement TaI-DPT \cite{guo2022texts} from the official code as a baseline, and apply the feature surgery on its predictions to verify the complementarity of our method. 

For the interactive segmentation, we convert text to points for the Segment Anything Model (SAM) \cite{kirillov2023segment}. It helps to replace the cost of manual labeling and avoids bad performance of SAM using text prompt only. Specifically, we pick points whose scores are higher than 0.8 from the similarity map, and take the same number of points ranked last as background points. Note, there is only one text prompt for SAM instead of multiple texts. Thus, we implement the feature surgery via the redundant feature $\boldsymbol{F}_{empty}$ from text features of an empty string to replace $expand(\boldsymbol{F}_r)$ in Eq. \ref{eq_feature_surgery}. This situation is the same to multimodal visualization, where the whole sentence is used as a text label without other categories. And we use the string ``[start][end]" (start flag and end flag, respectively) to extract redundant feature.

\begin{figure}[h]
\centering
 \includegraphics[width=8.3cm]{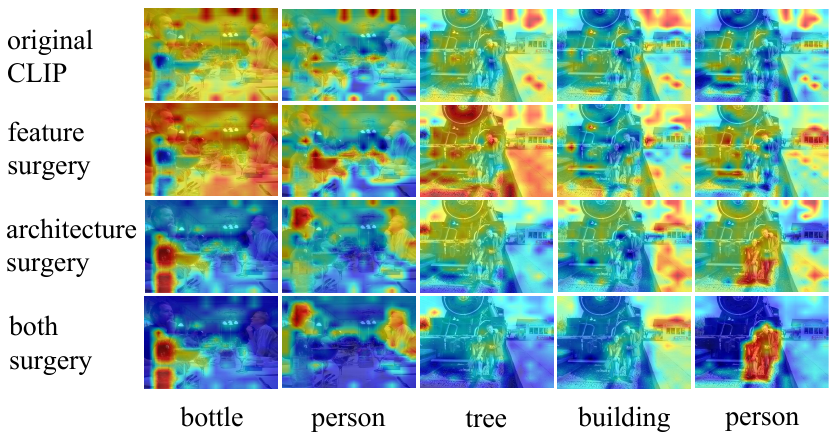}
\caption{Visual ablation study for individual modules and the combination (CLIP Surgery).}
\label{fig_vis_ablation}
\end{figure}

\begin{figure*}[h]
\centering
 \includegraphics[width=1\textwidth]{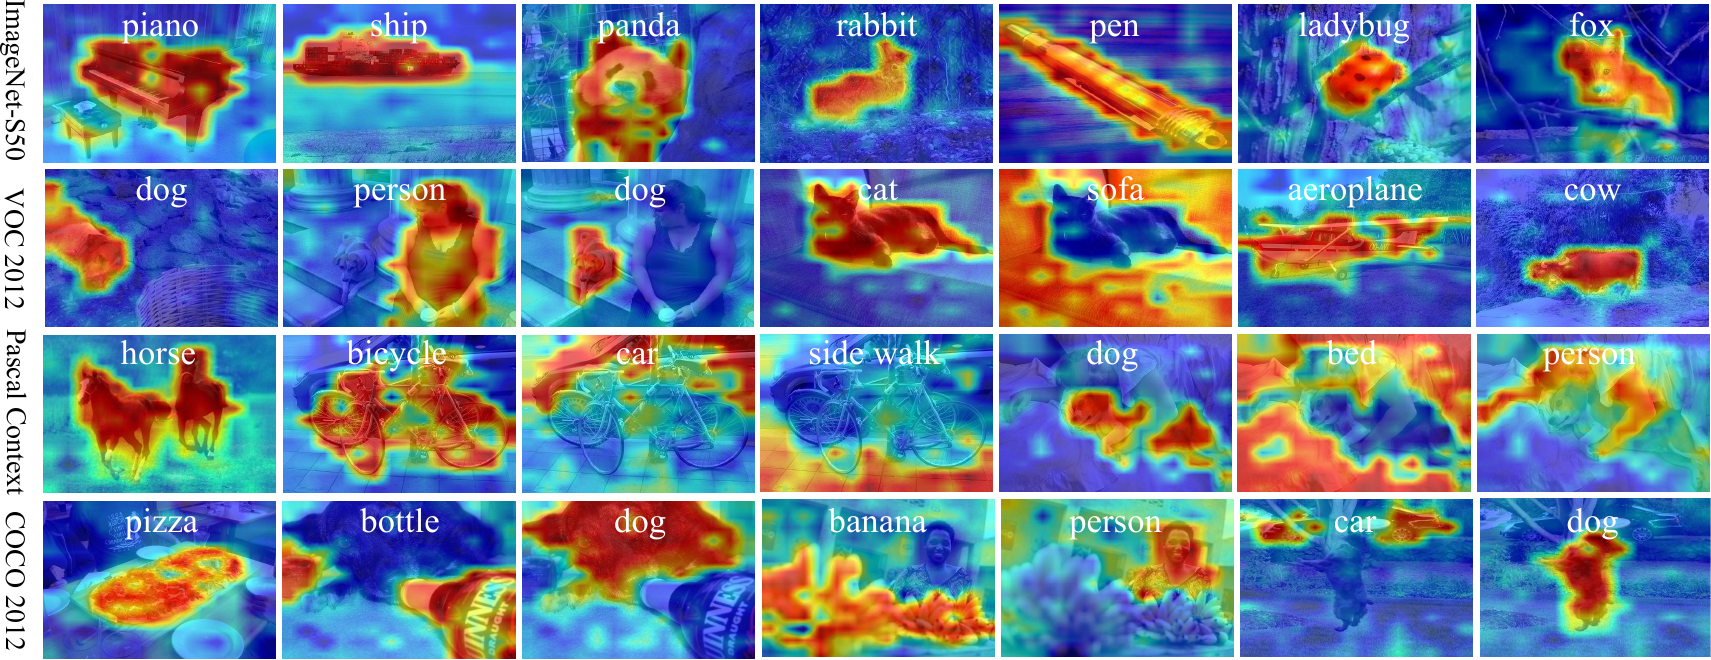}
\caption{Our CLIP Surgery solves the explainability problems, and provides good visualizations on varied datasets.}
\label{fig_vis_datasets}
\end{figure*}

\section{Visual Ablation Study} \label{sup6}

Besides the quantitative ablation study in Tab. \ref{tab_feature_surgery}, we provide the visual ablation results as Fig. \ref{fig_vis_ablation} to demonstrate the effectiveness of individual modules and the combination. Firstly, we depict the original similarity maps in the first row, whose results are opposite and noisy. Then we apply the feature surgery without architecture surgery as the second row. The opposite visualization still exists, while the common noises (see top regions of original CLIP) are mitigated and the results turn to be smoother. It indicates feature surgery can remove previews noises, while wrong similarity maps without architecture surgery lead to irregular noises. For architecture surgery only, the results become reasonable with fewer noises under improved similarity map. However, the common responses still exist in varied degree (see the train and right region in the last three columns). In the last row, the CLIP Surgery includes both modules, and the results are further improved based on the architecture surgery. Specifically, the high responses on the ceiling and table become darker in the first two columns, and the noises in the last three columns are obviously mitigated.

\section{Qualitative Results of Explainability Task} \label{sup7}

We present visualization results for different datasets in Fig. \ref{fig_vis_datasets}. The visualizations demonstrate that our proposed method effectively addresses the two discussed problems: opposite visualization and noisy activations. Notably, the proposed method enables us to produce clear and interpretable visualizations based solely on the original CLIP, without any additional training or complex back-propagation.

\section{Extensive Comparison with Previous Works} \label{sup8}

\begin{table*}[h]
\centering
\setlength\tabcolsep{7.5pt}
\begin{tabular}{ccccccccc}
\hline 
  &  \multicolumn{2}{c}{ImageNet-S50} &\multicolumn{2}{c}{VOC 2012} & \multicolumn{2}{c}{PASCAL Context} & \multicolumn{2}{c}{COCO 2017}\\
Method & mIoU $\uparrow$ & mSC $\uparrow$ & mIoU $\uparrow$ & mSC $\uparrow$ & mIoU $\uparrow$ & mSC $\uparrow$ & mIoU $\uparrow$ & mSC $\uparrow$ \\
\hline
\multicolumn{9}{c}{ResNet-50} \\
\cdashline{1-9}[0.5pt/5pt]
CLIP \cite{radford2021learning} & 28.18 & -26.50 & 17.78 & -27.88 & 16.98 & -14.02 & 10.53 & -19.17\\
Grad-CAM$^\star$ \cite{selvaraju2017grad} & 34.39 & 1.30 & 22.93 & 1.76 & 19.85 & 0.76 & 13.11 & 1.89 \\
pLRP$^\star$ \cite{lapuschkin2019unmasking} & - & - & - & - & - & - & - & - \\
Bi-Modal$^\star$ \cite{chefer2021generic} & - & - & - & - & - & - & - & - \\
gScoreCAM$^\star$ \cite{chen2022gscorecam} & 62.21 & 33.80 & 48.53 & 33.69 & 34.68 & 23.27 & 12.98 & 13.32 \\
RCLIP \cite{li2022exploring} & 54.45 & 26.50 & 41.17 & 27.88 & 28.48 & 14.02 & 21.87 & 19.17 \\
ECLIP\dag \cite{li2022exploring} & 62.49 & 30.49 & 50.04 & 31.14 & 36.28 & 21.77 & 27.27 & 23.43 \\
\textbf{CLIP Surgery (Ours)} & \textbf{66.05} & \textbf{43.28} & \textbf{53.85} & \textbf{44.60} & \textbf{38.50} & \textbf{32.44} & \textbf{29.24} & \textbf{33.80} \\
\hline
\multicolumn{9}{c}{ViT-B/16} \\
\cdashline{1-9}[0.5pt/5pt]
CLIP \cite{radford2021learning} & 27.87 & -18.84 & 17.36 & -19.86 & 15.76 & -16.73 & 9.74 & -23.37\\
Grad-CAM$^\star$ \cite{selvaraju2017grad} & 28.59 & -11.05 & 17.90 & -14.51 & 16.04 & -14.68 & 9.89 & -18.91 \\
pLRP$^\star$ \cite{lapuschkin2019unmasking} & 46.76 & 10.33 & 31.73 & 8.88 & 25.61 & 6.24 & 21.06 & 11.22 \\
Bi-Modal$^\star$ \cite{chefer2021generic} & 43.37 & 6.77 & 30.64 & 6.76 & 24.31 & 3.95 & 18.33 & 7.99 \\
gScoreCAM$^\star$ \cite{chen2022gscorecam} & 24.75 & 7.47 & 11.33 & 1.59 & 13.26 & 0.35 & 13.59 & 4.45 \\
RCLIP \cite{li2022exploring} & 48.00 & 16.14 & 37.36 & 18.51 & 33.25 & 18.21 & 26.12 & 22.41 \\
ECLIP\dag \cite{li2022exploring} & 58.59 & 26.32 & 48.46 & 28.83 & 30.34 & 14.43 & 24.67 & 18.95 \\
\textbf{CLIP Surgery (Ours)} & \textbf{62.41} & \textbf{36.50} & \textbf{55.78} & \textbf{41.64} & \textbf{46.28} & \textbf{34.32} & \textbf{35.23} & \textbf{35.43} \\
\hline 
\end{tabular}
\caption{\label{tab_comp_sota_sup} Results compared with previous state-of-the-art explainability methods. Besides, ``CLIP'' indicates the similarity map of CLIP. ```-'' means this method is not applicable to ResNet, ``\dag" notes the model requires extra fine-tuning, and ``$\star$" indicates that back-propagations are required for each label at lower efficiency. Note, mIoU (\%) measures the mean intersection over union for positive labels, and mSC indicates the mean score contrast in Eq. \ref{eq_msc}.}
\end{table*}

In this part, we compare the proposed CLIP Surgery with previous explainability works, including similarity map of original CLIP, Grad-CAM \cite{selvaraju2017grad} for CNN, pLRP \cite{lapuschkin2019unmasking} implemented by \cite{chefer2021transformer} for multiple layers, Bi-Modal \cite{chefer2021generic} based on ViT for multiple modalities, and explainability methods \cite{li2022exploring,chen2022gscorecam} for CLIP. We compare our method with them at the same backbone, ViT-B/16, and implement them from the official codebases. We list the results in Table \ref{tab_comp_sota_sup}. From this table, our CLIP Surgery archives the best performances on all datasets, metrics and backbones, also beyond other methods at large margins. For ViT-B/16, the second place is ECLIP \cite{li2022exploring} where the pooling is replaced with extra training, while our CLIP Surgery still surpasses it by max gains at 15.94\% mIoU and 19.89\% mSC without any training. Except our method, RCLIP \cite{li2022exploring} ranks first in the methods without extra training, and our results are significantly higher than it by 18.42\% at mIoU and 23.13\% at mSC. As for rest methods, their performances gap compared with ours are larger. Within them, Grad-CAM \cite{selvaraju2017grad} is similar to CLIP, showing the problem of opposite visualization. For ResNet-50, our results are still the best with obvious improvements. Especially, the mSC is higher than the second, ECLIP \cite{li2022exploring}, more than 10\%, even it requires extra fine-tuning. Notably, pLRP \cite{lapuschkin2019unmasking} and Bi-Modal \cite{chefer2021generic} are designed for ViT only and cannot be applied to ResNet, while gScoreCAM \cite{chen2022gscorecam} renders much worse results on ViT. Surpassing these methods, the proposed CLIP Surgery generalizes to varied backbones well besides good performance.

\begin{table}
\centering
\begin{tabular}{ccc}
\hline 
Method & VOC 2012 & PASCAL Context \\
\hline 
Grad-CAM \cite{selvaraju2017grad} & -0.93 & -0.72 \\
pLRP \cite{lapuschkin2019unmasking} & -7.15 & -4.27 \\
Bi-Modal \cite{chefer2021generic} & -3.53 & -2.04 \\
gScoreCAM \cite{chen2022gscorecam} & -11.98 & -8.14 \\
RCLIP \cite{li2022exploring} & -3.11 & \textbf{2.51} \\
ECLIP \cite{li2022exploring} & -1.31 & -7.64 \\
\textbf{CLIP Surgery} & \textbf{4.64} & \textbf{1.24} \\
\hline 
\end{tabular}
\caption{\label{tab_comp_limitation} Limitation of output size. Most methods except ours show worse results for higher output size, where the mIoU difference between ViT-B/16 (side 14) and ViT-B/32 (side 7) is lower than 0. Positive results are marked in bold.}
\end{table}

We observe another problem from Tab. \ref{tab_comp_sota_sup}, where the results of gScoreCAM \cite{chen2022gscorecam} are bad, even it's designed for CLIP. One reason is that it's not suitable for ViT, besides, it's owning to the limitation of output size. As shown in Tab. \ref{tab_comp_limitation}, most methods meet a performance drop when the output size is scaled up from 7 (ViT-B/32) to 14 (ViT-B/16). Within these methods, gScoreCAM is the most obvious method where the performances drop most for higher output size. It means it works better in lower output size, and it's highly limited at output size. This problem is easy to explain, because the min side of highlight is $\frac{1}{7}$ of ViT-B/32, and it reduces half for ViT-B/16. Thus, methods which focus on local region highlight less area, with worse results. While our method is not limited by the output size or patch size, and our results are higher when the model is scaled up. This finding suggests our method is applicable to tasks requiring dense predictions like segmentation.

\begin{figure*}[h]
\centering
 \includegraphics[width=1.\textwidth]{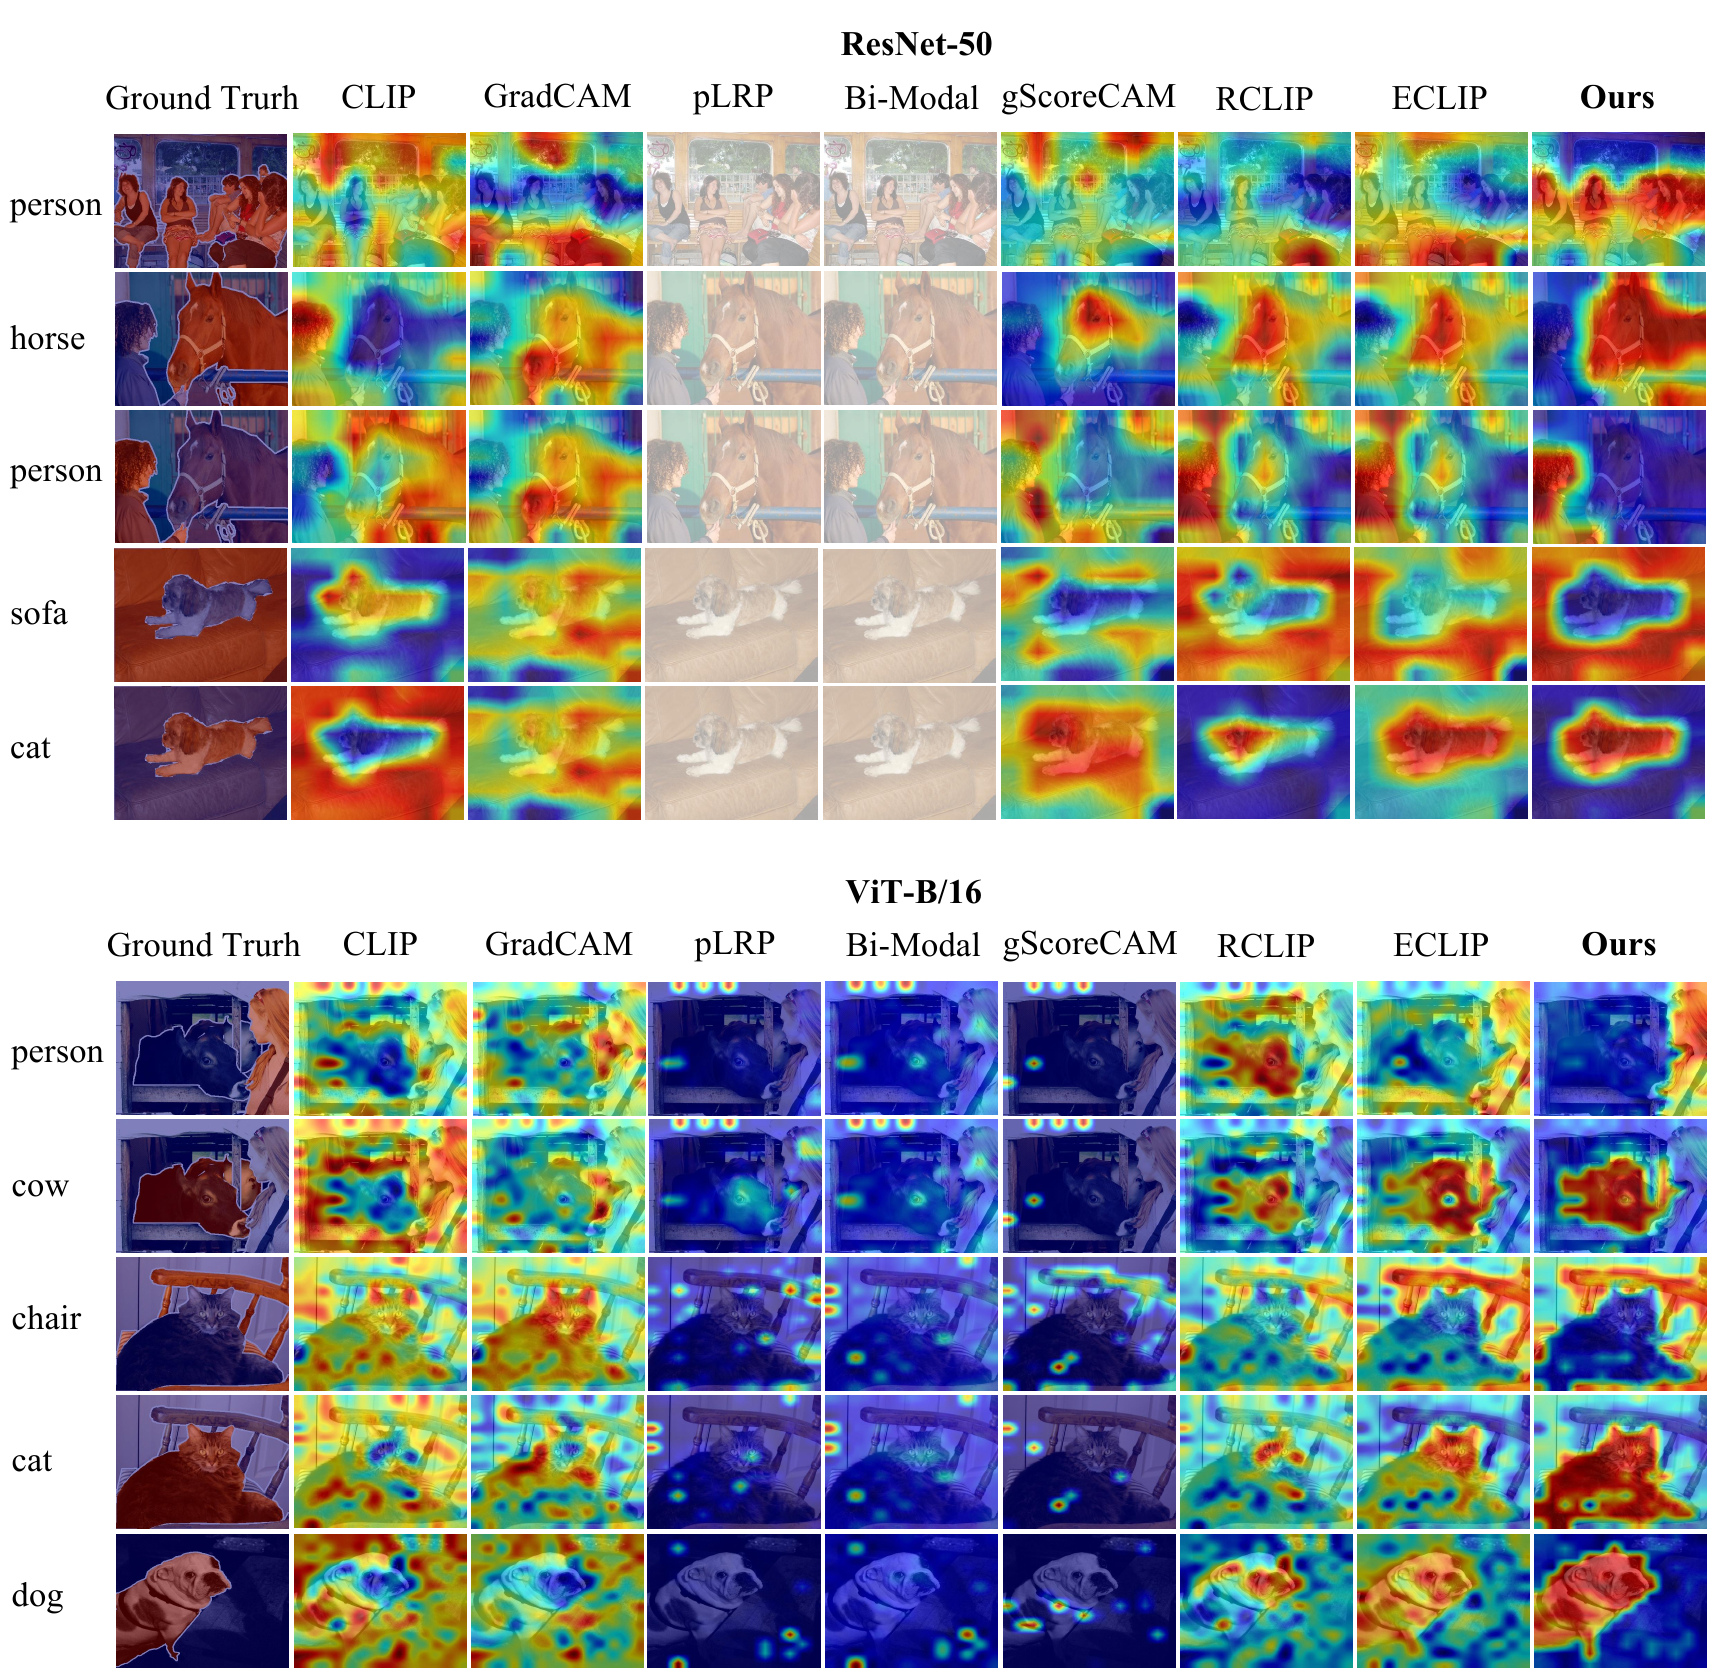}
\caption{Visual comparison between our CLIP Surgery with state-of-the-art explainability methods on VOC 2012 \cite{everingham2010pascal}. Note the foregrounds are colored in red, and the white mask indicates this method is not applicable to this backbone. Our visualization quality is much better than other methods for both ResNet and ViT, without any fine-tuning like ECLIP \cite{li2022exploring} or back-propagation in GradCAM \cite{selvaraju2017grad}. Besides, our method is not limited by certain backbone as pLRP \cite{lapuschkin2019unmasking}, Bi-Modal \cite{chefer2021generic} and gScoreCAM \cite{chen2022gscorecam}.}
\label{fig_vis_comp_sup}
\end{figure*}

In addition to the quantitative comparison, we also present a visual comparison in Fig. \ref{fig_vis_comp_sup}. The results show that our CLIP Surgery provides better quality visualizations compared to existing explainability methods, without problems of opposite visualization. Furthermore, our method produces fewer noisy activations than methods like pLRP \cite{lapuschkin2019unmasking}, Bi-Modal \cite{chefer2021generic}, gScoreCAM \cite{chen2022gscorecam}. Also, our method shows more obvious score contrast than RCLIP and ECLIP \cite{li2022exploring} at better visualization quality. All the above improvements enhance the model's visual explainability and make it more credible. 

\vspace{10cm}
\section{Visual Results of Open-vocabulary Semantic Segmentation} \label{sup9}

Then We perform a visual comparison between our method and previous state-of-the-art method MaskCLIP \cite{zhou2022extract}, as shown in Fig. \ref{fig_vis_seg}. The visualizations across datasets demonstrate the effectiveness of our approach in handling complex scenes without the need for pixel-level annotation. Our explainability method is capable of transferring well to the segmentation task, as evidenced by these results.

\begin{figure*}[h]
\centering
 \includegraphics[width=1\textwidth]{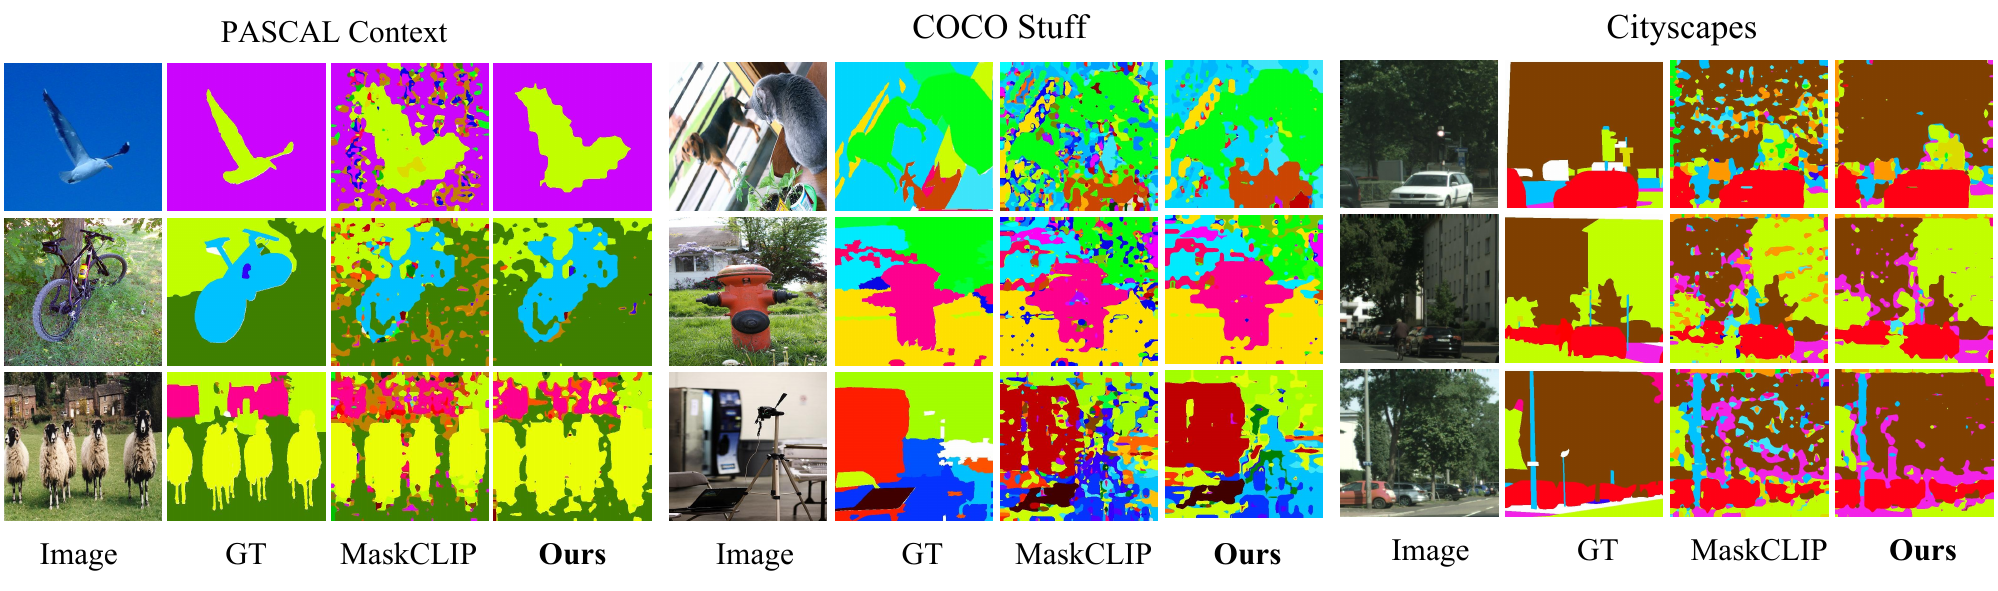}
\caption{Visual comparison of open-vocabulary semantic segmentation. We compare our CLIP Surgery with state-of-the-art methods MaskCLIP \cite{zhou2022extract} on PASCAL Context \cite{mottaghi2014role}, COCO stuff \cite{caesar2018coco} and patch of Cityscapes \cite{cordts2016cityscapes}, respectively. }
\label{fig_vis_seg}
\end{figure*}

\section{Activation Function in Open-vocabulary Multi-label Recognition} \label{sup10}

For multi-label recognition based on CLIP, we emphasize the importance of activation function and the effectiveness of our method. Unlike previous multi-label recognition methods supervised by fully supervisions, CLIP is sensitive to the final activation function to generate final scores, as shown in Tab. \ref{tab_comp_act}. The results of original cosine distance ``None" are similar to performances of sigmoid, which are obviously lower than softmax. Because, the contrastive loss of CLIP corresponds to softmax. For our method, we apply the CLIP feature surgery via replacing features of image tokens $\hat{F}_i$ to features of class token $F_c$ as described in the last paragraph of  Sec. \ref{sec_4.3}. It removes the redundant features with significant improvements on the evaluated datasets, where the gains at backbone ResNet-50 are 3.45\%, 4.41\% compared with the second on PASCAL Context \cite{mottaghi2014role} and NUS-Wide \cite{chua2009nus}, respectively. Also, the improvement is over 10\% compared with the original logit ``None" on PASCAL Context. All above results show the noticeable effectiveness of our approach.

\begin{table}[h]
\centering
\begin{tabular}{ccc}
\hline 
Method & PASCAL Context & NUS-Wide \\
\hline
\multicolumn{3}{c}{ResNet-50} \\
\cdashline{1-3}[0.5pt/5pt]
None & 36.91 & 32.75 \\
Sigmoid & 36.52 & 32.24 \\
Softmax & 43.90 & 35.58 \\
Ours & \textbf{47.35} & \textbf{39.99} \\
\hline 
\multicolumn{3}{c}{ViT-B/16} \\
\cdashline{1-3}[0.5pt/5pt]
None & 47.09 & 35.58 \\
Sigmoid & 47.09 & 40.39 \\
Softmax & 49.40 & 42.85 \\
Ours & \textbf{52.61} & \textbf{47.19} \\
\hline 
\end{tabular}
\caption{\label{tab_comp_act} Open-vocabulary multi-label recognition results with different activation operations.  ``None" indicates original cosine distance, and ``Ours" is the proposed CLIP Feature Surgery. The evaluation metric is mAP (\%).}
\end{table}

\section{More Results about Application on SAM} \label{sup11}

Interactive segmentation \cite{boykov2001interactive,rother2004grabcut,lempitsky2009image} is a classical computer vision task that involves segmenting a target object from an image with user guidance in the form of points, scribbles, or boxes during the inference phase. With the advent of large vision models, a recent work called the \textbf{Segment Anything Model (SAM)} \cite{kirillov2023segment} has made significant progress in enabling interactive segmentation via text prompts in an open-vocabulary manner. However, the SAM model performs poorly with text prompts alone, and the authors suggest combining text with manual points for better results. Our motivation is to replace the need for manual points entirely by using CLIP Surgery with text-only inputs. Our proposed method provides pixel-level results from text input, which can be readily converted to point prompts for the SAM model. Specifically, we select foreground points ranked ahead in the similarity map, and use the same number of points ranked last as background points.

When compared to other explainability methods, our CLIP Surgery offers two distinct advantages in converting text to points: (1) We have successfully mitigated the impact of noisy activations. As a result, the top points generated by our method are more reliable than those produced by other methods. (2) Our method is not limited by resolution, as demonstrated in Table \ref{tab_comp_limitation}. This enables us to increase resolution as needed to achieve better segmentation results.

Our solution offers several advantages over other prompt formats in SAM. (1) Our method requires text input only, without the annotation cost of manual points suggested in the paper of SAM (specifically, figure 12). (2) Point prompts are superior to mask prompts, because SAM's mask prompt is designed for its own output logits. This means that the generated points are more suitable than masks from another model. (3) Text to points is more readily achievable than the solution of text to boxes, because we only need CLIP without any fine-tuning. In contrast, open-vocabulary detection methods generate boxes requiring fine-tuning \cite{du2022learning}, and additional supervisions \cite{zhang2022glipv2} or models like proposal networks \cite{zhong2022regionclip} are usually needed.

\begin{figure}[h]
\centering
 \includegraphics[width=8.3cm]{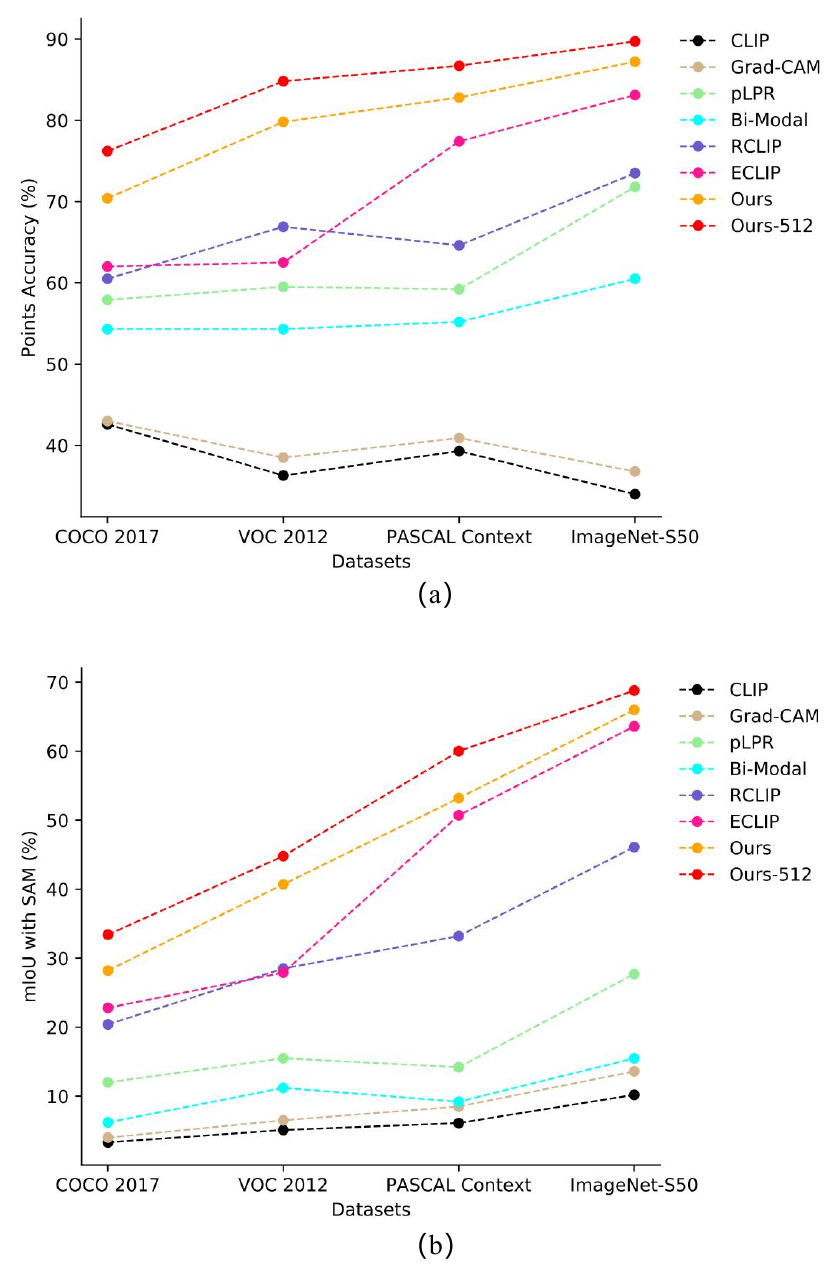}
\caption{Comparison of points accuracy (a) and mIoU with SAM \cite{kirillov2023segment} among explainability methods on four datasets. Note, all the input size is 224, except ``Ours-512" at 512.}
\label{fig_sam_ori}
\end{figure}

We focus to compare with other explainability methods in the solution of text to points. For all methods, we use the ViT-B/16 of CLIP as the backbone, with an input size of 224. Then, we select points with scores higher than 0.8 as positives, and use the same number of negatives ranked last as input prompts for the SAM. The accuracy of points and the mIoU after the SAM processing are plotted in Fig. \ref{fig_sam_ori}. Our method outperforms others in terms of both points accuracy and mIoU with SAM all four datasets. Specifically, We achieve points accuracies close to 90\% on some datasets, and the mIoU on ImageNet-S50 is approximately 70\%. Note that the mIoU is evaluated independently on each positive label.

\begin{table}[h]
\centering
\setlength\tabcolsep{2pt}
\begin{tabular}{cccc}
\hline 
Setting & Threshold & Point Acc. & mIoU \\
\hline
& 0.6 & 73.16 & 36.85 \\
& 0.65 & 74.86 & 38.12 \\
& 0.7 & 76.59 & 39.12 \\
224$\times$224 & 0.75 & 78.26 & 39.86 \\
with feature surgery & \textbf{0.8} & 79.83 & 40.70 \\
& 0.85 & 81.13 & 40.50 \\
& 0.9 & 82.44 & 39.60 \\
& 0.95 & 83.29 & 37.65 \\
\hline
wo. feature surgery & 0.8 & 77.65 & 38.78 \\
\hline 
512$\times$512 &\textbf{0.8} & \textbf{84.75} & \textbf{44.75} \\
\hline 
\end{tabular}
\caption{\label{tab_sam} Ablation study about threshold and the feature surgery for points selection on PASCAL Context dataset \cite{mottaghi2014role}.}
\end{table}

We have also included the results of our ablation study in Table \ref{tab_sam}. The table reveals that having a higher threshold results in higher points accuracy. However, a moderate threshold of 0.8 performs the best because a lower threshold introduces more points and maintains higher recall. Furthermore, increasing the input resolution significantly improves accuracy and mIoU. Notably, the feature surgery in not used in open-vocab. semantic segmentation, but it's helpful in this task.

\begin{figure}[h]
\centering
 \includegraphics[width=1.0\textwidth]{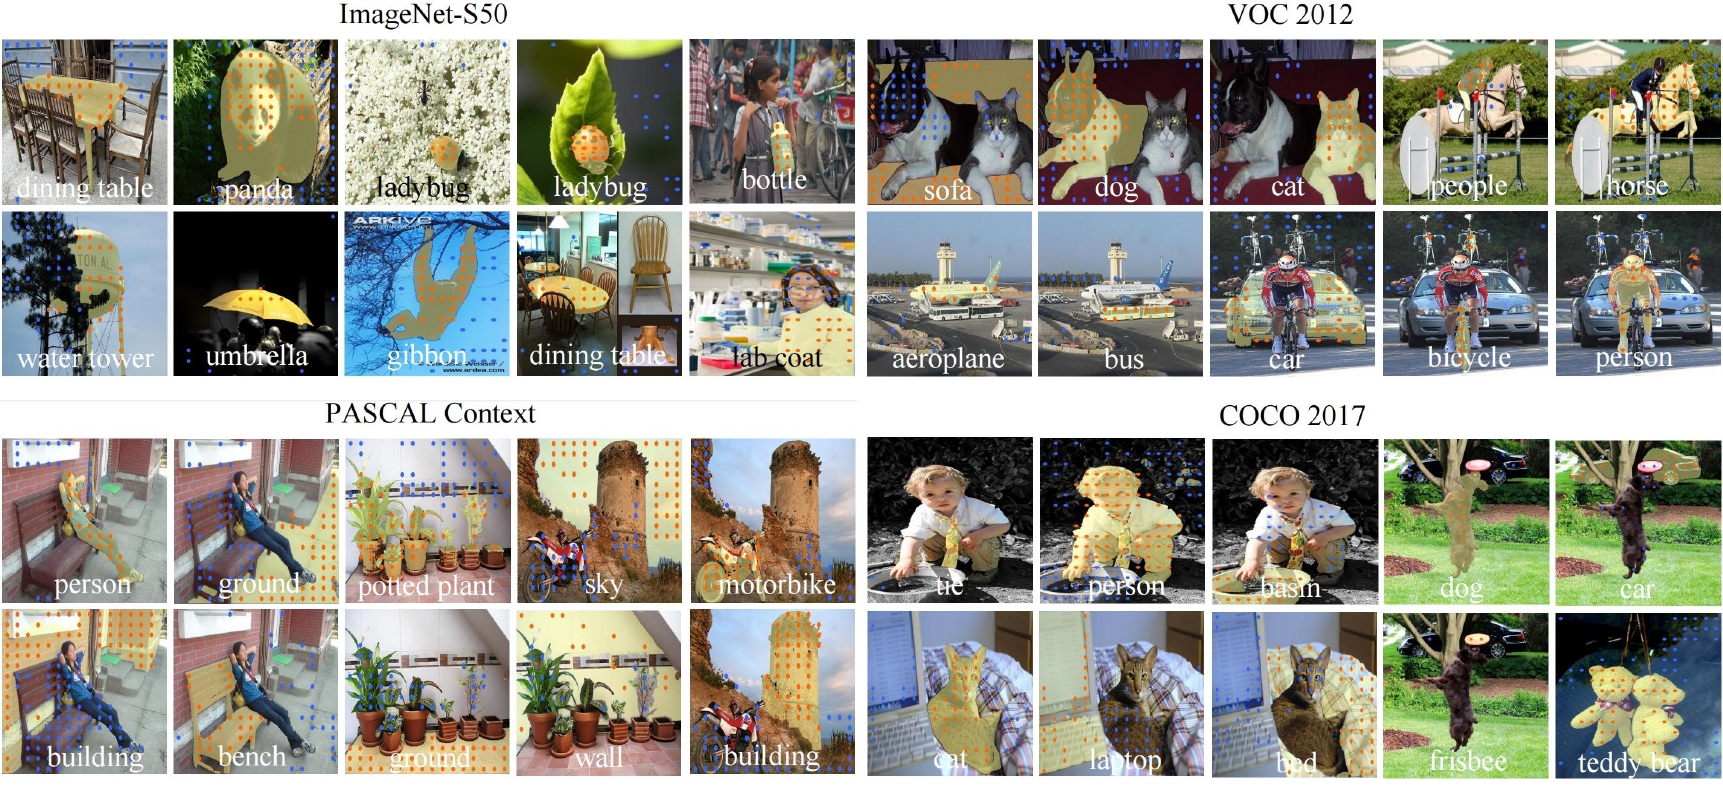}
\caption{Visualization of SAM \cite{kirillov2023segment} (yellow mask) using point prompts from our CLIP Surgery. The orange points indicate predicted foreground points and blue points mean the backgrounds.}
\label{fig_sam_vis_ori}
\end{figure}

We have also included visualizations of our results in Fig. \ref{fig_sam_vis_ori}. These visualizations showcase the predicted mask from SAM as well as the points prompt generated by our CLIP Surgery. Notably, we use the ViT-B/16 backbone at an input size of 512. The visualization results demonstrate that SAM guided by CLIP Surgery performs better than the similarity map or semantic segmentation results. In particular, the mask generated after SAM processing is impressive at the boundary with very few noisy pixels, resulting in a higher visual quality. Additionally, the points generated by our CLIP Surgery are accurate, indicating that our method is applicable and effective.

\begin{figure}[h]
\centering
 \includegraphics[width=8.3cm]{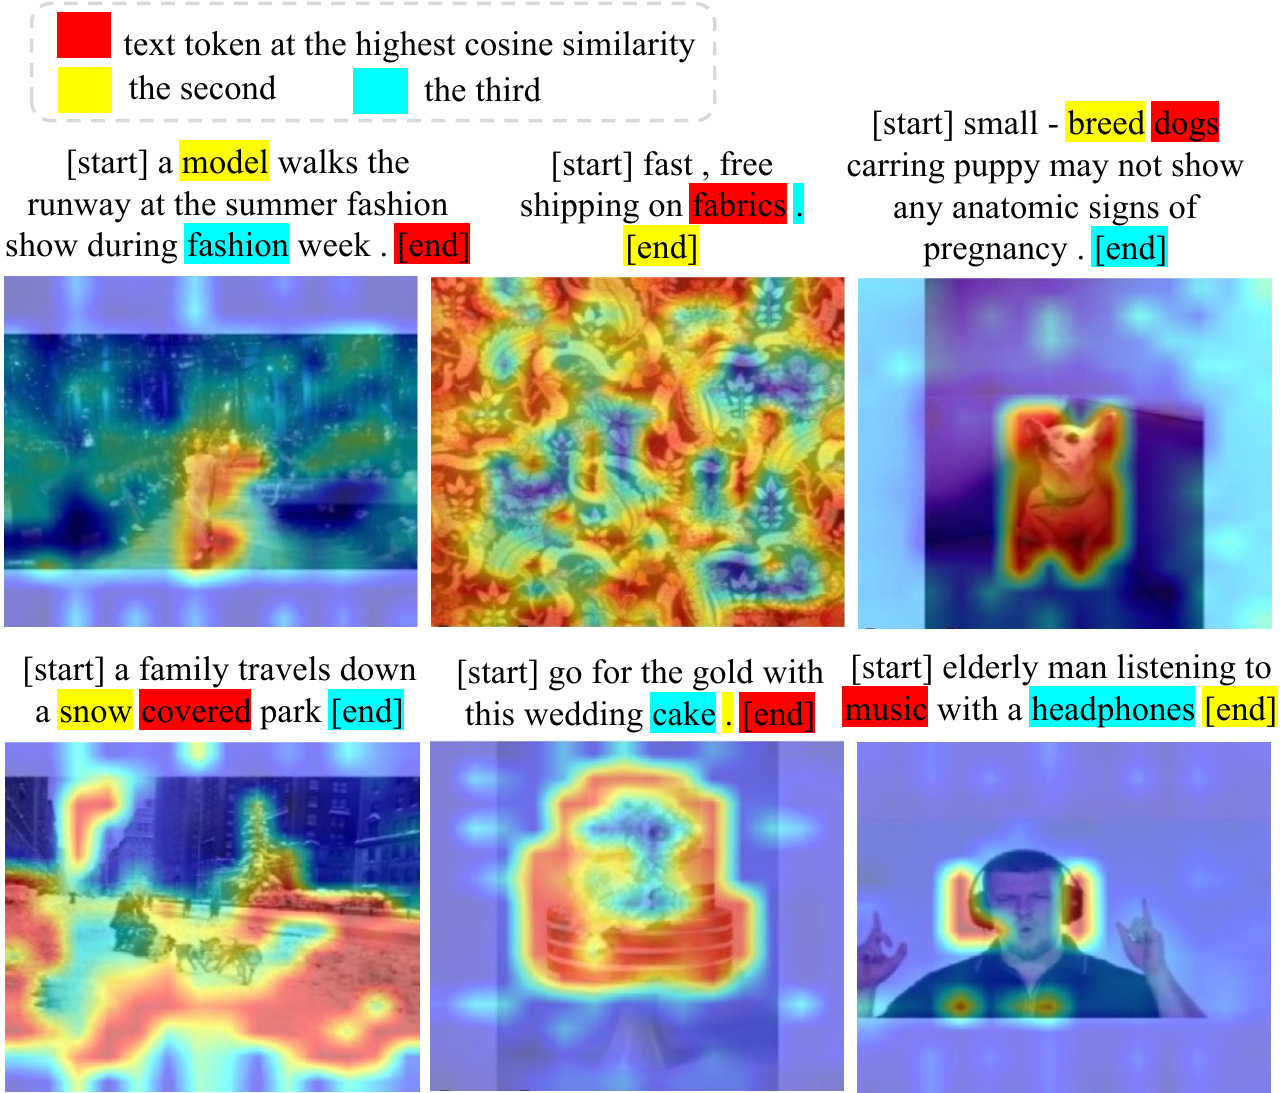}
\caption{Multimodal visualization to explain the image-text pairs used in the training process of CLIP. The visual explainability results are from the proposed CLIP Surgery, and textual explainability results are based on the cosine distance of each text token. [start] indicates the start text token and [end] means the end text token. Note, we mark the text token at the highest cosine similarly in red, then draw the second in yellow and blue for the third.}
\label{fig_vis_multimodal2}
\end{figure}

\section{Details and Extensive Examples of Multimodal Visualization} \label{sup12}

\begin{figure}[h]
\centering
 \includegraphics[width=0.9\textwidth]{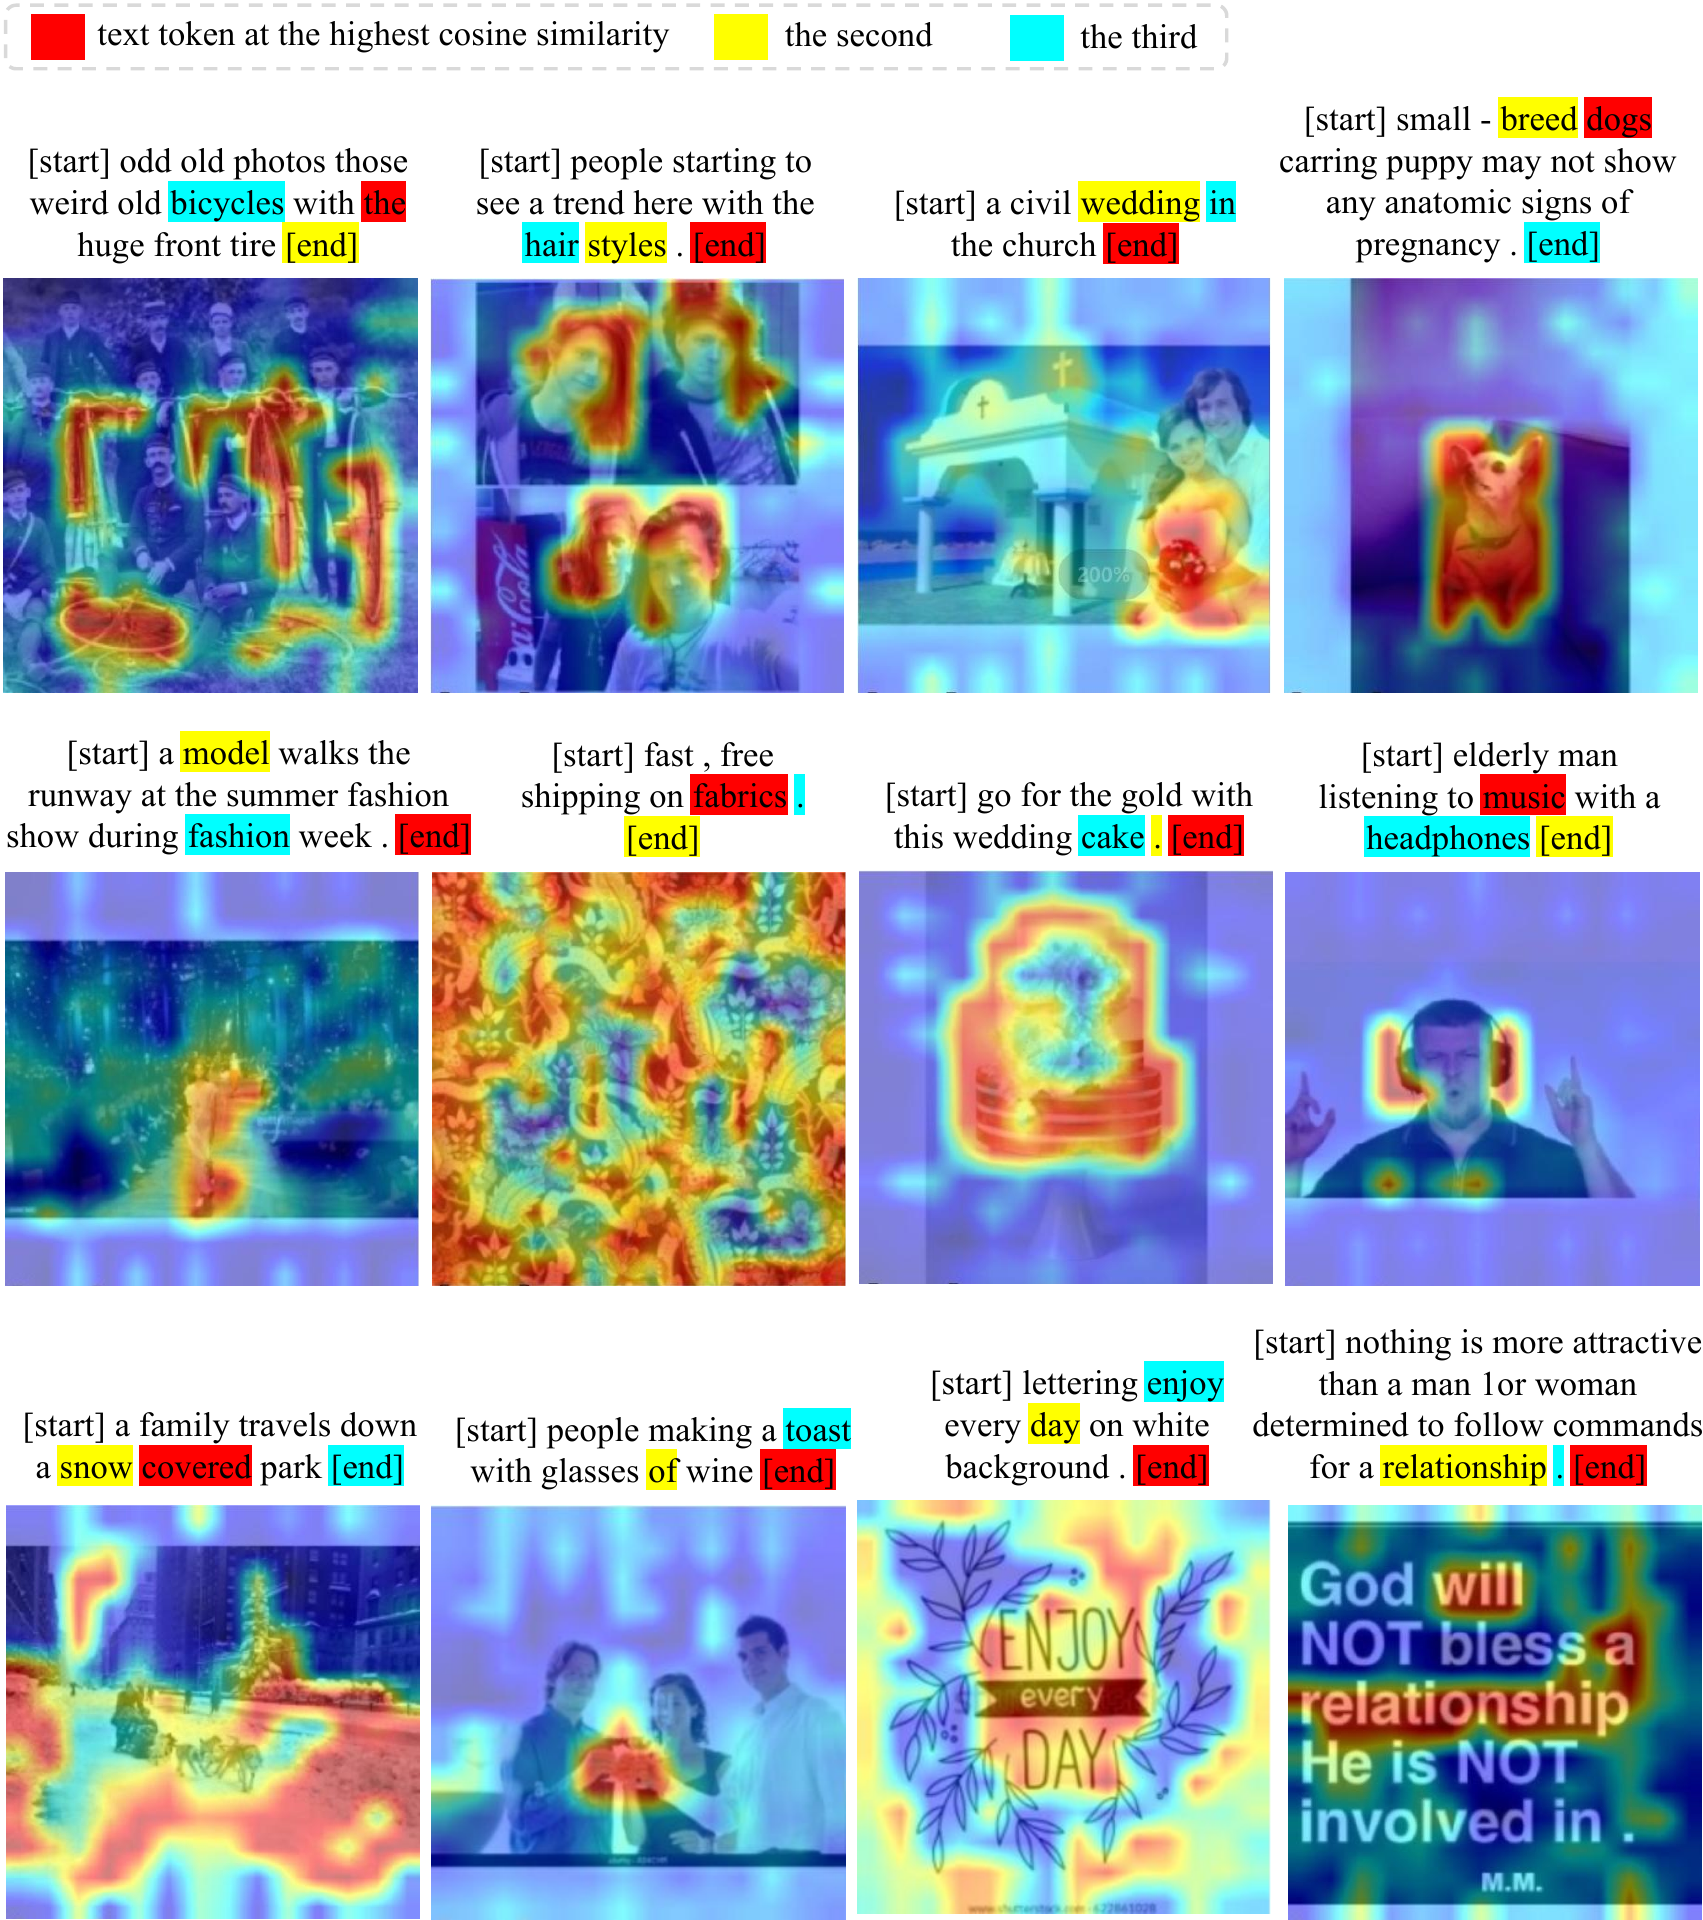}
\caption{Multimodal visualization to explain the image-text pairs used in the training process of CLIP. The visual explainability results are from the proposed CLIP Surgery, and textual explainability results are based on the cosine distance of each text token. [start] indicates the start text token and [end] means the end text token. Note, we mark the text token at the highest cosine similarly in red, then draw the second in yellow and blue for the third.}
\label{fig_vis_multimodal}
\end{figure}

Besides above visualization results on image modality for varied tasks, we also explain the learning process of CLIP by the multimodal visualization. Specifically, we visualize the image-text pairs during training, where the whole sentence is used as a textual label for visual explanation. At the same time, we show the top text tokens whose scores are ranked in front. For the implementation, we use image-text pairs (training data) from the GCC3M dataset \cite{sharma2018conceptual}, since the training data of CLIP is private and not available. Then we draw the similarity map via our CLIP Surgery method, and mark the high response text tokens. Specifically, the feature of class token $\boldsymbol{F_c}$ is used to compute similarity scores for each text token, and the text at max similarity is served for the generation of similarity map with image tokens $\boldsymbol{F_i}$. Note, there is only one sentence instead of multiple texts, thus we implement the feature surgery via the redundant feature $\boldsymbol{F}_{empty}$ from text features of an empty sentence ([start][end]) to replace $expand(\boldsymbol{F}_r)$ in Eq. \ref{eq_feature_surgery}. Besides. the backbone is ViT-B/16 at input resolution 224. Based on above implementation details, we draw multimodal visualization results as Fig. \ref{fig_vis_multimodal}.

From these multimodal visualization results, we observed some interesting phenomenons. For the visual results, we summarize two points: (1) Not all the objects or stuffs are highlighted in the image, because only the text token at the highest cosine similarity is picked for training (red texts in Fig. \ref{fig_vis_multimodal}). Thus, we believe CLIP learns partial context from one image. (2) CLIP is able to recognize the texts from an image in some extent, as shown in the last two images of Fig. \ref{fig_vis_multimodal}. Since the highlights are corresponded with text tokens (e.g., day, enjoy, relationship). For the textual visualization results, there are two findings: (1) The end token is the most common activated text token, and some non-object words are at high response too (e.g., ``in", ``.", ``of"). It means the text encoder of CLIP embeds the information of whole sentences in certain words. (2) The object-based words also occurs frequently with corresponding salient objects in the image. While their cosine similarities often ranks second or third behind the end token ``[end]". These findings are interesting, also they reveal some characteristics of image-text pairs of CLIP, thus provides potential value to further improvement of CLIP's training process.

\clearpage
